# Supplementary material for: Nonlocal energy density functionals for pairing and beyond-mean-field calculations
Source: arXiv:1611.09311 source file (2017-02-11)
Supplement: Supplementary file 1 [file reg_pairing-supp-01.pdf]

# Supplemental material for: Nonlocal energy density functionals for pairing and beyond-mean-field calculations

**K. Bennaceur[1,2,3], A. Idini[2,4], J. Dobaczewski[2,3,5,6], P. Dobaczewski[7], M. Kortelainen[2,3], and F. Raimondi[2,4]**

[1]Université de Lyon, F-69003 Lyon, France; Institut de Physique Nucléaire de Lyon, CNRS/IN2P3, Université Lyon 1, F-69622 Villeurbanne Cedex, France

[2]Department of Physics, PO Box 35 (YFL), FI-40014 University of Jyväskylä, Finland

[3]Helsinki Institute of Physics, P.O. Box 64, FI-00014 University of Helsinki, Finland

[4]Department of Physics, University of Surrey, Guildford GU2 7XH, United Kingdom

[5]Department of Physics, University of York, Heslington, York YO10 5DD, United Kingdom

[6]Institute of Theoretical Physics, Faculty of Physics, University of Warsaw, ul. Hoża 69, PL-00681 Warsaw, Poland

[7]ul. Obozowa 85 m. 5, PL-01425 Warsaw, Poland

## 1. Covariance matrices

In files:
REG2c.161026.covariance.matrix.five.eigenvalues.kept.txt
REG4c.161026.covariance.matrix.five.eigenvalues.kept.txt
we give the NLO and N$^2$LO covariance matrices calculated for five largest eigenvalues kept in the Hessian matrices. The order of coupling constants is the same as that shown in columns denoted by REG2c.161026 and REG4c.161026, respectively, in Table 3 of the article.

## 2. Coupling constants

In Figs. 1–7, we show coupling constants of the adjusted NLO and N$^2$LO pseudopotentials as functions of the regularization range $a$.

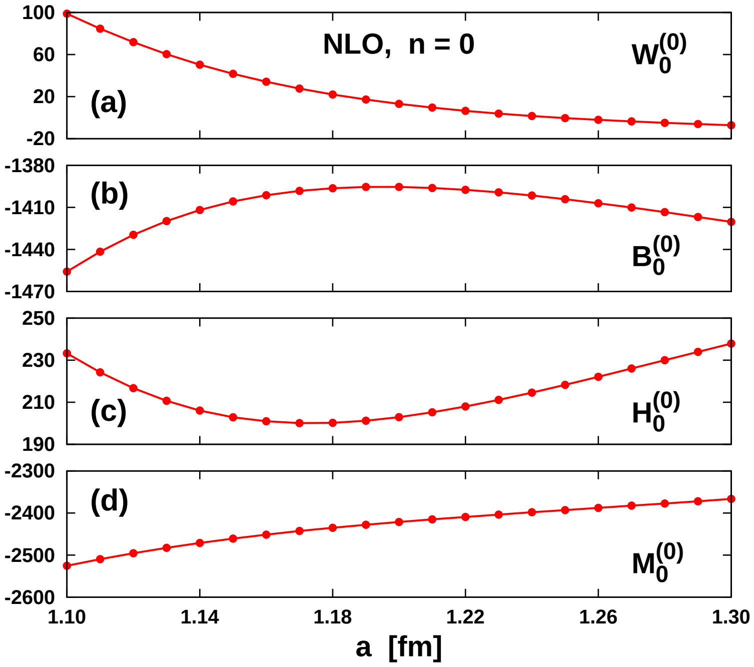


**Figure 1.** (Color online) Coupling constants $W_1^{(0)}$, $B_1^{(0)}$, $H_1^{(0)}$, and $M_1^{(0)}$ of the NLO pseudopotential as functions of the regularization range $a$.

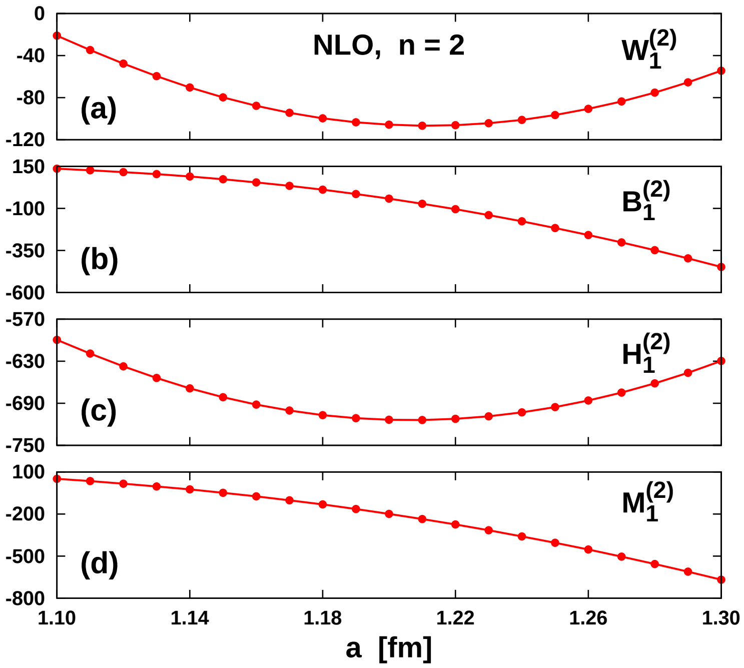


**Figure 2.** (Color online) Coupling constants $W_1^{(2)}$, $B_1^{(2)}$, $H_1^{(2)}$, and $M_1^{(2)}$ of the NLO pseudopotential as functions of the regularization range $a$.

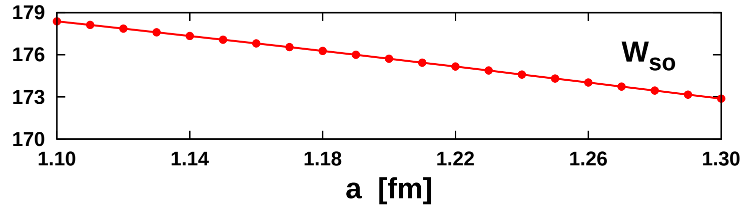


**Figure 3.** (Color online) The spin-orbit coupling constant $W_{\rm SO}$ of the NLO pseudopotential as a function of the regularization range $a$.

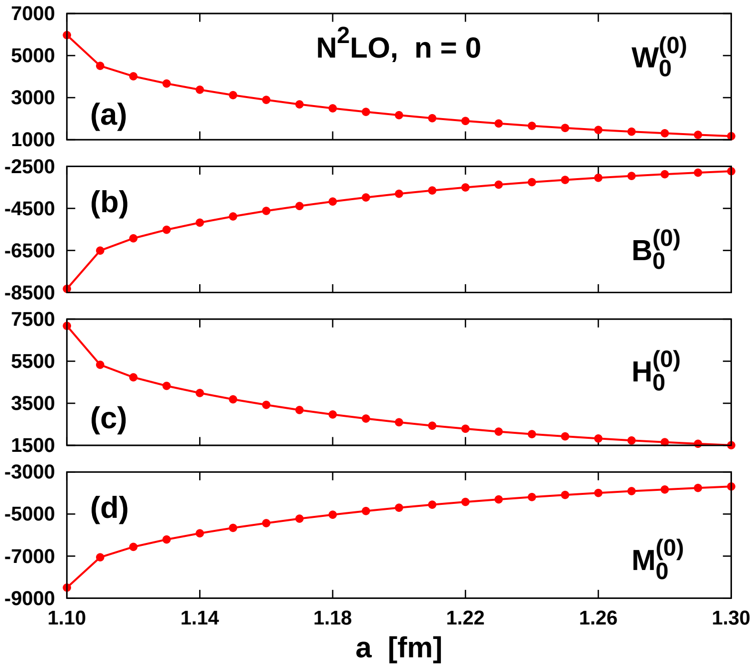


**Figure 4.** (Color online) Coupling constants $W_1^{(0)}$, $B_1^{(0)}$, $H_1^{(0)}$, and $M_1^{(0)}$ of the N$^2$LO pseudopotential as functions of the regularization range $a$.

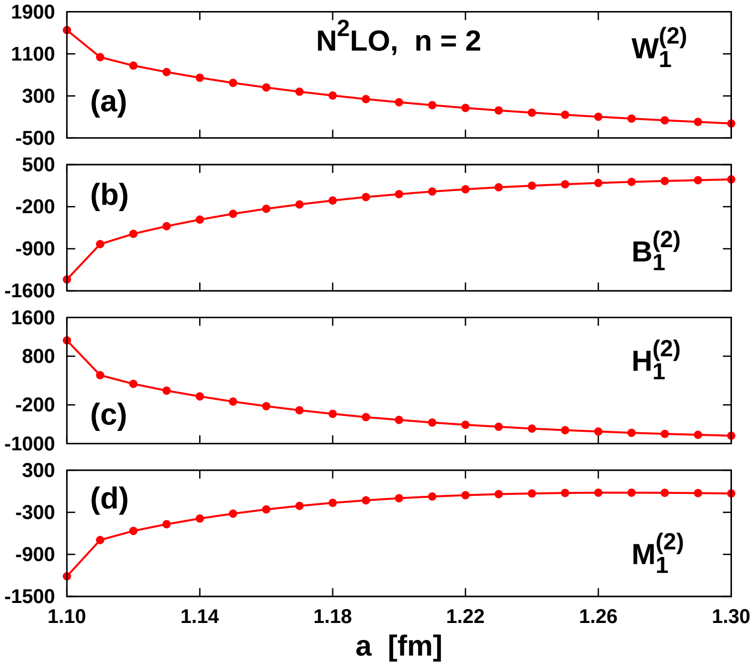


**Figure 5.** (Color online) Coupling constants $W_1^{(2)}$, $B_1^{(2)}$, $H_1^{(2)}$, and $M_1^{(2)}$ of the N$^2$LO pseudopotential as functions of the regularization range $a$.

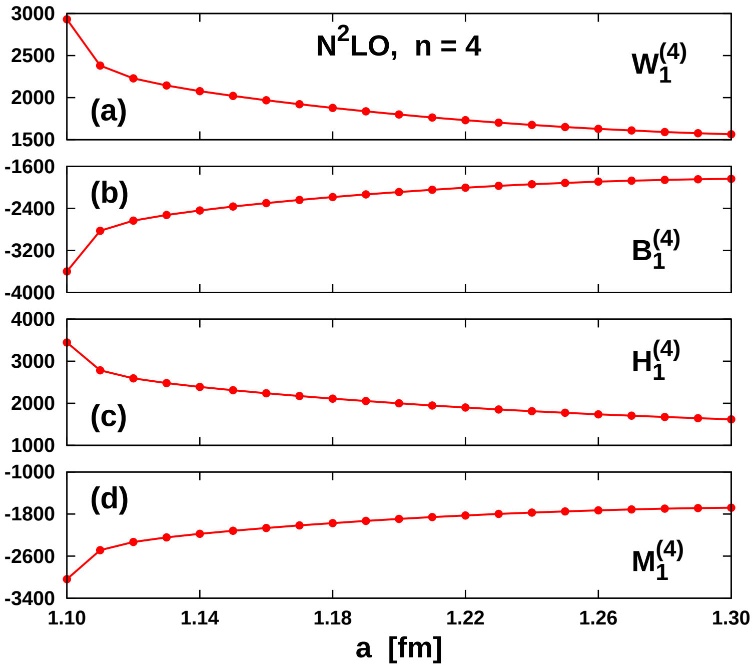


**Figure 6.** (Color online) Coupling constants $W_1^{(4)}$, $B_1^{(4)}$, $H_1^{(4)}$, and $M_1^{(4)}$ of the N$^2$LO pseudopotential as functions of the regularization range $a$.

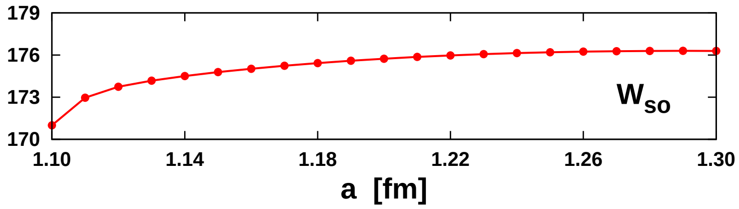


**Figure 7.** (Color online) The spin-orbit coupling constant $W_{\rm SO}$ of the N$^2$LO pseudopotential as a function of the regularization range $a$.
